# Supplementary material for: Quantum logic for state preparation, readout, and leakage detection with binary subspace measurements
Source: arXiv:2410.23531 source file (2024-10-31)
Supplement: Supplementary file 1 [file appendix.tex]

\documentclass[aps,pra,twocolumn,showpacs,superscriptaddress,groupedaddress]{revtex4}
\usepackage{graphicx}    % needed for figures
\usepackage{dcolumn}    % needed for some tables
\usepackage{bm}             % for math
\usepackage{amssymb}   % for math
\usepackage{amsmath}    % for multiline equation
\usepackage{subfigure}    % for subfigure
\usepackage{braket}
\usepackage{mathrsfs}
\usepackage[font=small,labelfont=bf]{caption}
\usepackage[toc,page]{appendix}
\hyphenation{ALPGEN}
\hyphenation{EVTGEN}
\hyphenation{PYTHIA}

\appendix
\begin{appendices}

\\ \\

\end{appendices}
